# Supplementary material for: A Tutte-Like Theorem for Injective Flows on Meshes
Source: arXiv:2610.30149 source file (2026-08-06)
Supplement: Supplementary file 1 [file appendix-proofs.tex]

\subsection{Index Theorem on genus 0}\label{proof:gortler}
\begin{definition}\label{def:ind_classification}
    The index of a vertex $\vertx \in \verts$ is $\ind{\vertx} = (2-\signchg{\vertx})/2$, where $\signchg{\vertx}$ is the number of sign changes in the values of $(\harmfunc_{\vertx'} - \harmfunc_{\vertx})$ as one traverses all the $\vertx'$ in the ordered one-ring of $\vertx$. 
    % $v$ is called a non-singular vertex if $ind(v)=0$ and a saddle vertex if $ind(v)<0$. If $ind(v)=1$, and all values of $\Delta z$ at $v$ are positive, $v$ is called a source, otherwise $v$ is called a sink. \newline
    The index of a face $\tri \in \tris$ is $\ind{f} = (2-\signchg{f})/2$, where $\signchg{f}$ is the number of sign changes in the values of $\Delta z$ as one traverses the half edges of $\partial f$ in order. $f$ is called a non-singular face if $ind(f)=0$ and a saddle face if $ind(f)<0$. If $ind(f)=1$, $f$ is called a vortex.

\end{definition}
